# Supplementary material for: Reconstructing massive quivers on a defect circle
Source: arXiv:2611.34129 source file (2026-11-25)
Supplement: Supplementary file 1 [file appendix_b_cylinder_helpers.tex]

\newcommand{\Bcylbase}[1]{%
\path[fill=#1](-1.3,0)--(-1.3,4.6)arc(180:0:1.3 and .36)--(1.3,0)arc(0:-180:1.3 and .36)--cycle;
}
\newcommand{\Bcylshell}{%
\draw[gray!65,line width=.55pt](-1.3,0)--(-1.3,4.6)(1.3,0)--(1.3,4.6);
\draw[gray!65,line width=.55pt,dashed](1.3,0)arc(0:180:1.3 and .36);
\draw[gray!65,line width=.55pt](-1.3,0)arc(180:360:1.3 and .36);
\fill[white](0,4.6)ellipse(1.3 and .36);\draw[gray!65,line width=.55pt](0,4.6)ellipse(1.3 and .36);
}
\newcommand{\Bxloop}{%
\draw[bc,line width=1.15pt,dashed](1.3,2.3)arc(0:180:1.3 and .36);
\draw[bc,line width=1.15pt](-1.3,2.3)arc(180:360:1.3 and .36);
\draw[bc,->,line width=1.15pt](-1.19,2.155)..controls(-1.10,2.10)and(-.99,2.06)..(-.90,2.04);
\node[left,bc]at(-1.35,2.38){$X_x$};
}
\newcommand{\Bparticle}{%
\draw[ic,line width=1.2pt,->](.88,-.265)--(.88,4.79)node[above right]{$\alpha=X_i$};
\filldraw[fill=white,draw=ic,line width=.75pt](.88,2.035)circle(.055);
}
\newcommand{\Bdefect}{%
\draw[xc,line width=1.2pt,->](0,-.36)--(0,4.79)node[above left]{$X_1$};
\filldraw[fill=white,draw=black,line width=.8pt](0,1.94)circle(.145);\node at(0,1.94){\scriptsize$c$};
}
