# Supplementary material for: Reconstructing massive quivers on a defect circle
Source: arXiv:2611.34129 source file (2026-11-25)
Supplement: Supplementary file 2 [file appendix_b_d_helpers.tex]

% Complete cut-annulus networks. The two square a ports are the two
% ends of ONE vacuum strand cut open at a fixed spatial cut.
% Canonical two-vertex fusion tree, with the same straight, parallel
% branches as the main-text blocks. The bottom/top vacuum ports are paired.
\newcommand{\standardbasisblock}[2]{%
\begin{scope}[shift={(.5,1.3)}]
\draw(0,0)--(0,.55)--(.85,1.65)--(0,2.75);
\draw[xc](0,.55)--(-1.7,2.75);
\draw[ic](.85,1.65)--(1.7,2.75);
\fill(0,.55)circle(1.6pt)(.85,1.65)circle(1.6pt);
\node[right=3pt]at(.48,1.08){$v_{#2}$};
\path(-2.05,-.4)rectangle(2.05,3.5);
\foreach \p in {(0,0),(0,2.75)}{\filldraw[fill=white,draw=black]\p rectangle ++(.12,.12);}
\node[below]at(0,-.05){$v_{#1}$};\node[above]at(0,2.87){$v_{#1}$};
\node[above,xc]at(-1.7,2.75){$X_1$};\node[above,ic]at(1.7,2.75){$X_i$};
\end{scope}}
\newcommand{\rawinputstate}{\standardbasisblock{u}{v}}
\newcommand{\standardoutputstate}{\standardbasisblock{a}{b}}
\newcommand{\unresolvedaction}{%
\draw(.8,0)--(.8,.8)--(1.5,3.4)--(.8,6);
\draw[bc](-.8,0)..controls(-.8,1.6)and(-1.05,2.4)..(-.4,3);
\draw[xc](.8,.8)--(-.4,3);
\draw(-.4,3)--(-.4,3.5);
\draw[xc](-.4,3.5)..controls(-1.1,4.1)and(-1.2,5.0)..(-1.2,6);
\draw[bc](-.4,3.5)..controls(.4,4.1)and(.15,5.0)..(.15,6);
\draw[ic](1.5,3.4)--(2.2,6);
\fill(.8,.8)circle(1.6pt)(1.5,3.4)circle(1.6pt)(-.4,3)circle(1.6pt)(-.4,3.5)circle(1.6pt);
\node[right]at(.8,.35){$v_u$};\node[right]at(1.18,2.2){$v_v$};\node[left]at(-.4,3.23){$X_c$};
\node[right,xc]at(-.05,2.35){$X_1$};
\path(-1.65,-.45)rectangle(2.7,6.55);
\foreach \p in {(-.8,0),(.8,0),(.15,6),(.8,6)}{\filldraw[fill=white,draw=black]\p rectangle ++(.12,.12);}
\node[below,bc]at(-.8,-.05){$X_x$};\node[above left,bc]at(.15,6.12){$X_x$};
\node[below]at(.8,-.05){$v_u$};\node[above right]at(.8,6.12){$v_u$};
\node[above,xc]at(-1.2,6){$X_1$};\node[above,ic]at(2.2,6){$X_i$};}
\newcommand{\cutports}{%
\path(-1.65,-.45)rectangle(2.7,6.55);
\foreach \p in {(0,0),(.7,6)}{\filldraw[fill=white,draw=black]\p rectangle ++(.12,.12);}
\node[below]at(0,-.05){$v_a$};\node[above]at(.7,6.12){$v_a$};
\node[above,xc]at(-1.2,6){$X_1$};\node[above,ic]at(2.2,6){$X_i$};}
\newcommand{\netcommon}{%
\draw[xc]plot[smooth,tension=.5]coordinates{(-.4,3.5)(-1.2,4.15)(-1.2,6)};
\draw[bc]plot[smooth,tension=.5]coordinates{(-.4,3.5)(.4,4.15)(.7,5.2)};
\draw plot[smooth,tension=.5]coordinates{(1.6,4)(1,4.7)(.7,5.2)(.7,6)};
\draw[ic]plot[smooth,tension=.5]coordinates{(1.6,4)(2.2,4.7)(2.2,6)};
\node[left,bc]at(.4,4.45){$X_x$};\node[right]at(1,4.7){$v_u$};
\node[right]at(1.6,3.3){$v_v$};
\fill(-.4,3.5)circle(1.6pt)(1.6,4)circle(1.6pt)(.7,5.2)circle(1.6pt);}
\newcommand{\wholeinitial}{%
\draw plot[smooth,tension=.5]coordinates{(0,0)(0,.5)(.8,1.05)(.8,1.7)};
\draw[bc]plot[smooth,tension=.5]coordinates{(0,.5)(-.8,1.05)(-.8,2.25)(-.4,3)};
\draw[xc]plot[smooth,tension=.5]coordinates{(.8,1.7)(-.1,2.35)(-.4,3)};
\draw plot[smooth,tension=.5]coordinates{(.8,1.7)(1.6,2.35)(1.6,4)};
\draw(-.4,3)--(-.4,3.5);
\node[right]at(.8,1.25){$v_u$};\node[left,bc]at(-.8,1.8){$X_x$};
\node[right,xc]at(-.1,2.35){$X_1$};\node[left]at(-.4,3.23){$X_c$};
\fill(0,.5)circle(1.6pt)(.8,1.7)circle(1.6pt)(-.4,3)circle(1.6pt);
\netcommon}
\newcommand{\wholefirstF}{%
\draw plot[smooth,tension=.5]coordinates{(0,0)(0,.5)(-.4,1.05)(-.4,1.65)};
\draw plot[smooth,tension=.5]coordinates{(0,.5)(1.6,2.35)(1.6,4)};
\draw[bc](-.4,1.65)..controls(-1.15,2.05)and(-1.15,2.6)..(-.4,3);
\draw[xc](-.4,1.65)..controls(.35,2.05)and(.35,2.6)..(-.4,3);
\draw(-.4,3)--(-.4,3.5);
\node[left]at(-.4,1.25){$X_t$};\node[left]at(-.4,3.23){$X_c$};
\node[left,bc]at(-.96,2.3){$X_x$};\node[right,xc]at(.16,2.3){$X_1$};
\fill(0,.5)circle(1.6pt)(-.4,1.65)circle(1.6pt)(-.4,3)circle(1.6pt);
\netcommon}
\newcommand{\wholeselected}{%
\draw plot[smooth,tension=.5]coordinates{(0,0)(0,.5)(-.4,3.5)};
\draw plot[smooth,tension=.5]coordinates{(0,.5)(1.6,2.35)(1.6,4)};
\node[left]at(-.18,1.95){$X_c$};\fill(0,.5)circle(1.6pt);
\netcommon}
\newcommand{\wholesecondF}{%
\draw plot[smooth,tension=.5]coordinates{(0,0)(0,.5)(.8,2.4)};
\draw[xc]plot[smooth,tension=.5]coordinates{(0,.5)(-1.2,2.1)(-1.2,6)};
\draw[bc]plot[smooth,tension=.5]coordinates{(.8,2.4)(.4,3.1)(.7,5.2)};
\draw plot[smooth,tension=.5]coordinates{(.8,2.4)(1.6,3.1)(1.6,4)(1,4.7)(.7,5.2)(.7,6)};
\draw[ic]plot[smooth,tension=.5]coordinates{(1.6,4)(2.2,4.7)(2.2,6)};
\node[right]at(.4,1.4){$v_b$};\node[left,bc]at(.4,3.8){$X_x$};
\node[right]at(1.6,3.45){$v_v$};\node[right]at(1,4.7){$v_u$};
\fill(0,.5)circle(1.6pt)(.8,2.4)circle(1.6pt)(1.6,4)circle(1.6pt)(.7,5.2)circle(1.6pt);}
\newcommand{\wholethirdF}{%
\draw plot[smooth,tension=.5]coordinates{(0,0)(0,.5)(.8,2.4)(.4,3.1)(.4,3.6)};
\draw[xc]plot[smooth,tension=.5]coordinates{(0,.5)(-1.2,2.1)(-1.2,6)};
\draw[ic]plot[smooth,tension=.5]coordinates{(.8,2.4)(2.2,3.7)(2.2,6)};
\draw[bc](.4,3.6)..controls(-.4,4.05)and(-.4,4.75)..(.4,5.2);
\draw(.4,3.6)..controls(1.2,4.05)and(1.2,4.75)..(.4,5.2);
\draw plot[smooth,tension=.5]coordinates{(.4,5.2)(.7,5.55)(.7,6)};
\node[right]at(.4,1.4){$v_b$};\node[left]at(.4,3.22){$v_{a'}$};
\node[left,bc]at(-.2,4.4){$X_x$};\node[right]at(1,4.4){$v_u$};
\node[right]at(.61,5.55){$v_a$};
\fill(0,.5)circle(1.6pt)(.8,2.4)circle(1.6pt)(.4,3.6)circle(1.6pt)(.4,5.2)circle(1.6pt);}
\newcommand{\wholeoutput}{%
\draw(0,0)--(0,1.4)--(.7,3.3)--(.7,6);
\draw[xc](0,1.4)--(-1.2,6);
\draw[ic](.7,3.3)--(2.2,6);
\node[right]at(.43,2.35){$v_b$};
\fill(0,1.4)circle(1.6pt)(.7,3.3)circle(1.6pt);}
\newcommand{\inputcutstate}{%
\begin{tikzpicture}[x=.68cm,y=.68cm,line width=.9pt,baseline=(current bounding box.center)]
\draw(0,0)--(0,.55)--(.65,1.45)--(.65,2.05)--(.35,3.1);
\draw[xc](0,.55)--(-1.05,1.9)--(-1.05,3.1);
\draw[ic](.65,1.45)--(1.55,2.1)--(1.55,3.1);
\fill(0,.55)circle(1.6pt)(.65,1.45)circle(1.6pt);
\node[right]at(.4,1){$v_v$};\node[below]at(0,0){$v_u$};\node[above]at(.35,3.1){$v_u$};
\node[above,xc]at(-1.05,3.1){$X_1$};\node[above,ic]at(1.55,3.1){$X_i$};
\path(-1.45,-.35)rectangle(1.95,3.7);
\node[font=\scriptsize,gray]at(.3,-.7){identified $v_u$ ports};
\end{tikzpicture}}
\newcommand{\cutidentity}{%
\begin{tikzpicture}[x=.72cm,y=.72cm,line width=.9pt,baseline=(current bounding box.center)]
\draw[bc](-.65,-1.2)--(-.65,1.2);\draw(.65,-1.2)--(.65,1.2);
\node[below,bc]at(-.65,-1.2){$X_x$};\node[above,bc]at(-.65,1.2){$X_x$};
\node[below]at(.65,-1.2){$v_u$};\node[above]at(.65,1.2){$v_u$};
\end{tikzpicture}}
\newcommand{\cutresolution}{%
\begin{tikzpicture}[x=.72cm,y=.72cm,line width=.9pt,baseline=(current bounding box.center)]
\draw[bc](-.65,-1.2)--(0,-.45);\draw(.65,-1.2)--(0,-.45);
\draw(0,-.45)--(0,.45);
\draw[bc](0,.45)--(-.65,1.2);\draw(0,.45)--(.65,1.2);
\fill(0,-.45)circle(1.6pt)(0,.45)circle(1.6pt);
\node[left]at(0,0){$v_a$};
\node[below,bc]at(-.65,-1.2){$X_x$};\node[above,bc]at(-.65,1.2){$X_x$};
\node[below]at(.65,-1.2){$v_u$};\node[above]at(.65,1.2){$v_u$};
\end{tikzpicture}}
